# Supplementary material for: Canonical formulation for the thermodynamics of $sl_n$-invariant integrable spin chains
Source: arXiv:2311.02238 source file (2023-11-03)
Supplement: Supplementary file 1 [file NLIEsl5a_sm.pdf]

# *Supplemental material for*
# "Canonical formulation for the thermodynamics of $sl_n$-invariant integrable spin chains"

I. R. Passos and A. Klümper
*Department of Physics, University of Wuppertal, Gaußstraße 20, 42119 Wuppertal, Germany*

T. S. Tavares
*Department of Physics, University of Wuppertal, Gaußstraße 20, 42119 Wuppertal, Germany*
*Departamento de Física, Universidade Federal de São Carlos, 13565-905 São Carlos-SP, Brazil*

In this note we apply the techniques introduced in the main text of the paper with the main example of $sl_4$ at hand to the somewhat more complicated case of $sl_5$. We present the adjacency matrices for this case as well as their corresponding graphical representations. We use them to identify the EAF's that appear in the expressions of auxiliary functions in Eqs.(4.57a)–(4.60d).

For the first representation the diagram is quite simple, leading to the adjacency matrix

$$A_{1,1}^{(5)}(x) = \begin{bmatrix} 0 & q_1^{(0)} & 0 & 0 & 0 \\ q_1^{(0)} & 0 & q_2^{(0)} & 0 & 0 \\ 0 & q_2^{(0)} & 0 & q_3^{(0)} & 0 \\ 0 & 0 & q_3^{(0)} & 0 & q_4^{(0)} \\ 0 & 0 & 0 & q_4^{(0)} & 0 \end{bmatrix}, \tag{S-1}$$

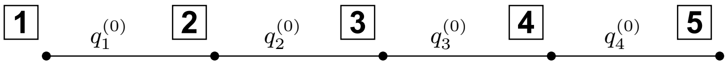


Figure S-1. Pole canceling graph of $sl_5$ for $a = 1$.

from which we obtain the factorization resp. the definition of the polynomials $p_{1,j}^{(5)}(x)$

$$\boxed{1,2} = \frac{\Phi_+(x)p_{1,1}^{(5)}(x)}{q_2(x)}, \qquad \boxed{2,3} = \frac{\Phi_+(x)\Phi_-(x)p_{1,2}^{(5)}(x)}{q_1(x)q_3(x)}, \qquad \boxed{3,4} = \frac{\Phi_+(x)\Phi_-(x)p_{1,3}^{(5)}(x)}{q_2(x)q_4(x)},$$

$$\boxed{1,3} = \frac{\Phi_+(x)p_{1,4}^{(5)}(x)}{q_3(x)}, \qquad \boxed{2,4} = \frac{\Phi_+(x)\Phi_-(x)p_{1,5}^{(5)}(x)}{q_1(x)q_4(x)}, \tag{S-2}$$

$$\boxed{4,5} = \frac{\Phi_-(x)p_{1,6}^{(5)}(x)}{q_3(x)}, \qquad \boxed{3,5} = \frac{\Phi_-(x)p_{1,7}^{(5)}(x)}{q_2(x)}, \qquad \boxed{1,4} = \frac{\Phi_+(x)p_{1,8}^{(5)}(x)}{q_4(x)}, \qquad \boxed{2,5} = \frac{\Phi_-(x)p_{1,9}^{(5)}(x)}{q_1(x)}. \tag{S-3}$$

Since it is straightforward to extract the subgraphs corresponding to these polynomials from Fig.S-1 we refrain to do so here. Note the polynomials Eqs.(S-2) and (S-6) have already appeared in the $sl_4$ case (see Eqs.(2.12)where however $q_4(x) = \Phi_+(x)$).

As for the second representation, see Fig.S-2, it follows

$$A^{(5)}_{2,1}(x)=\begin{bmatrix}
0 & q_2^{(1/2)} & 0 & 0 & 0 & 0 & 0 & 0 & 0 & 0\\
q_2^{(1/2)} & 0 & q_3^{(1/2)} & 0 & q_1^{(-1/2)} & 0 & 0 & 0 & 0 & 0\\
0 & q_3^{(1/2)} & 0 & q_4^{(1/2)} & 0 & q_1^{(-1/2)} & 0 & 0 & 0 & 0\\
0 & 0 & q_4^{(1/2)} & 0 & 0 & 0 & q_1^{(-1/2)} & 0 & 0 & 0\\
0 & q_1^{(-1/2)} & 0 & 0 & 0 & q_3^{(1/2)} & 0 & 0 & 0 & 0\\
0 & 0 & q_1^{(-1/2)} & 0 & q_3^{(1/2)} & 0 & q_4^{(1/2)} & q_2^{(-1/2)} & 0 & 0\\
0 & 0 & 0 & q_1^{(-1/2)} & 0 & q_4^{(1/2)} & 0 & 0 & q_2^{(-1/2)} & 0\\
0 & 0 & 0 & 0 & 0 & q_2^{(-1/2)} & 0 & 0 & q_4^{(1/2)} & 0\\
0 & 0 & 0 & 0 & 0 & 0 & q_2^{(-1/2)} & q_4^{(1/2)} & 0 & q_3^{(-1/2)}\\
0 & 0 & 0 & 0 & 0 & 0 & 0 & 0 & q_3^{(-1/2)} & 0
\end{bmatrix}, \tag{S-4}$$

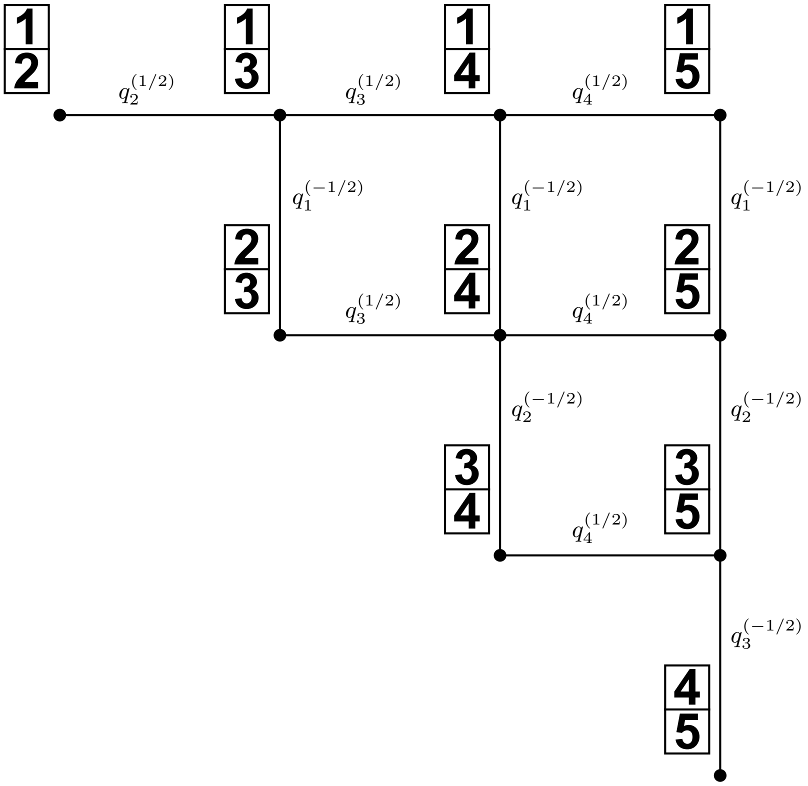


Figure S-2. Pole canceling graph of $sl_5$ for $a=2$.

providing

$$\begin{array}{|c|}\hline 1,2\\\hline 2,3\\\hline\end{array}=\frac{\Phi_+\left(x+\frac{\mathrm{i}}{2}\right)\Phi_-\left(x+\frac{\mathrm{i}}{2}\right)\Phi_+\left(x-\frac{\mathrm{i}}{2}\right)p^{(5)}_{2,1}(x)}{q_3\left(x+\frac{\mathrm{i}}{2}\right)},\quad \begin{array}{|c|}\hline 1,2\\\hline 2,4\\\hline\end{array}=\frac{\Phi_+\left(x+\frac{\mathrm{i}}{2}\right)\Phi_-\left(x+\frac{\mathrm{i}}{2}\right)\Phi_+\left(x-\frac{\mathrm{i}}{2}\right)p^{(5)}_{2,2}(x)}{q_2\left(x-\frac{\mathrm{i}}{2}\right)q_4\left(x+\frac{\mathrm{i}}{2}\right)}, \tag{S-5}$$

$$\begin{array}{|c|}\hline 1,3\\\hline 3,4\\\hline\end{array}=\frac{\Phi_+\left(x+\frac{\mathrm{i}}{2}\right)\Phi_-\left(x+\frac{\mathrm{i}}{2}\right)\Phi_+\left(x-\frac{\mathrm{i}}{2}\right)p^{(5)}_{2,3}(x)}{q_2\left(x+\frac{\mathrm{i}}{2}\right)q_4\left(x+\frac{\mathrm{i}}{2}\right)},\quad \begin{array}{|c|}\hline 2,3\\\hline 3,4\\\hline\end{array}=\frac{\Phi_+\left(x+\frac{\mathrm{i}}{2}\right)\Phi_-\left(x+\frac{\mathrm{i}}{2}\right)\Phi_+\left(x-\frac{\mathrm{i}}{2}\right)\Phi_-\left(x-\frac{\mathrm{i}}{2}\right)p^{(5)}_{2,4}(x)}{q_1\left(x-\frac{\mathrm{i}}{2}\right)q_4\left(x+\frac{\mathrm{i}}{2}\right)}, \tag{S-6}$$

also common to $sl_4$ (Eqs.(4.13)), and

$$
\begin{array}{|c|}\hline 3,4\\\hline 4,5\\\hline\end{array}=\frac{\Phi_+\left(x-\frac{\mathrm{i}}{2}\right)\Phi_-\left(x-\frac{\mathrm{i}}{2}\right)\Phi_-\left(x+\frac{\mathrm{i}}{2}\right)p^{(5)}_{2,5}(x)}{q_2\left(x-\frac{\mathrm{i}}{2}\right)},\qquad
\begin{array}{|c|}\hline 2,3\\\hline 3,5\\\hline\end{array}=\frac{\Phi_+\left(x-\frac{\mathrm{i}}{2}\right)\Phi_-\left(x-\frac{\mathrm{i}}{2}\right)\Phi_-\left(x+\frac{\mathrm{i}}{2}\right)p^{(5)}_{2,6}(x)}{q_1\left(x-\frac{\mathrm{i}}{2}\right)q_3\left(x-\frac{\mathrm{i}}{2}\right)},\tag{S-7}
$$

$$
\begin{array}{|c|}\hline 2,4\\\hline 4,5\\\hline\end{array}=\frac{\Phi_+\left(x-\frac{\mathrm{i}}{2}\right)\Phi_-\left(x-\frac{\mathrm{i}}{2}\right)\Phi_-\left(x+\frac{\mathrm{i}}{2}\right)p^{(5)}_{2,7}(x)}{q_1\left(x-\frac{\mathrm{i}}{2}\right)q_3\left(x+\frac{\mathrm{i}}{2}\right)},\qquad
\begin{array}{|c|}\hline 1,2\\\hline 2,5\\\hline\end{array}=\frac{\Phi_+\left(x-\frac{\mathrm{i}}{2}\right)\Phi_-\left(x+\frac{\mathrm{i}}{2}\right)p^{(5)}_{2,8}(x)}{q_2\left(x-\frac{\mathrm{i}}{2}\right)},\tag{S-8}
$$

$$
\begin{array}{|c|}\hline 1,4\\\hline 4,5\\\hline\end{array}=\frac{\Phi_+\left(x-\frac{\mathrm{i}}{2}\right)\Phi_-\left(x+\frac{\mathrm{i}}{2}\right)p^{(5)}_{2,9}(x)}{q_3\left(x+\frac{\mathrm{i}}{2}\right)},\qquad
\begin{array}{|c|}\hline 1,3\\\hline 3,5\\\hline\end{array}=\frac{\Phi_+\left(x-\frac{\mathrm{i}}{2}\right)\Phi_-\left(x+\frac{\mathrm{i}}{2}\right)p^{(5)}_{2,10}(x)}{q_2\left(x+\frac{\mathrm{i}}{2}\right)q_3\left(x-\frac{\mathrm{i}}{2}\right)},\tag{S-9}
$$

which are depicted in Fig.S-3.

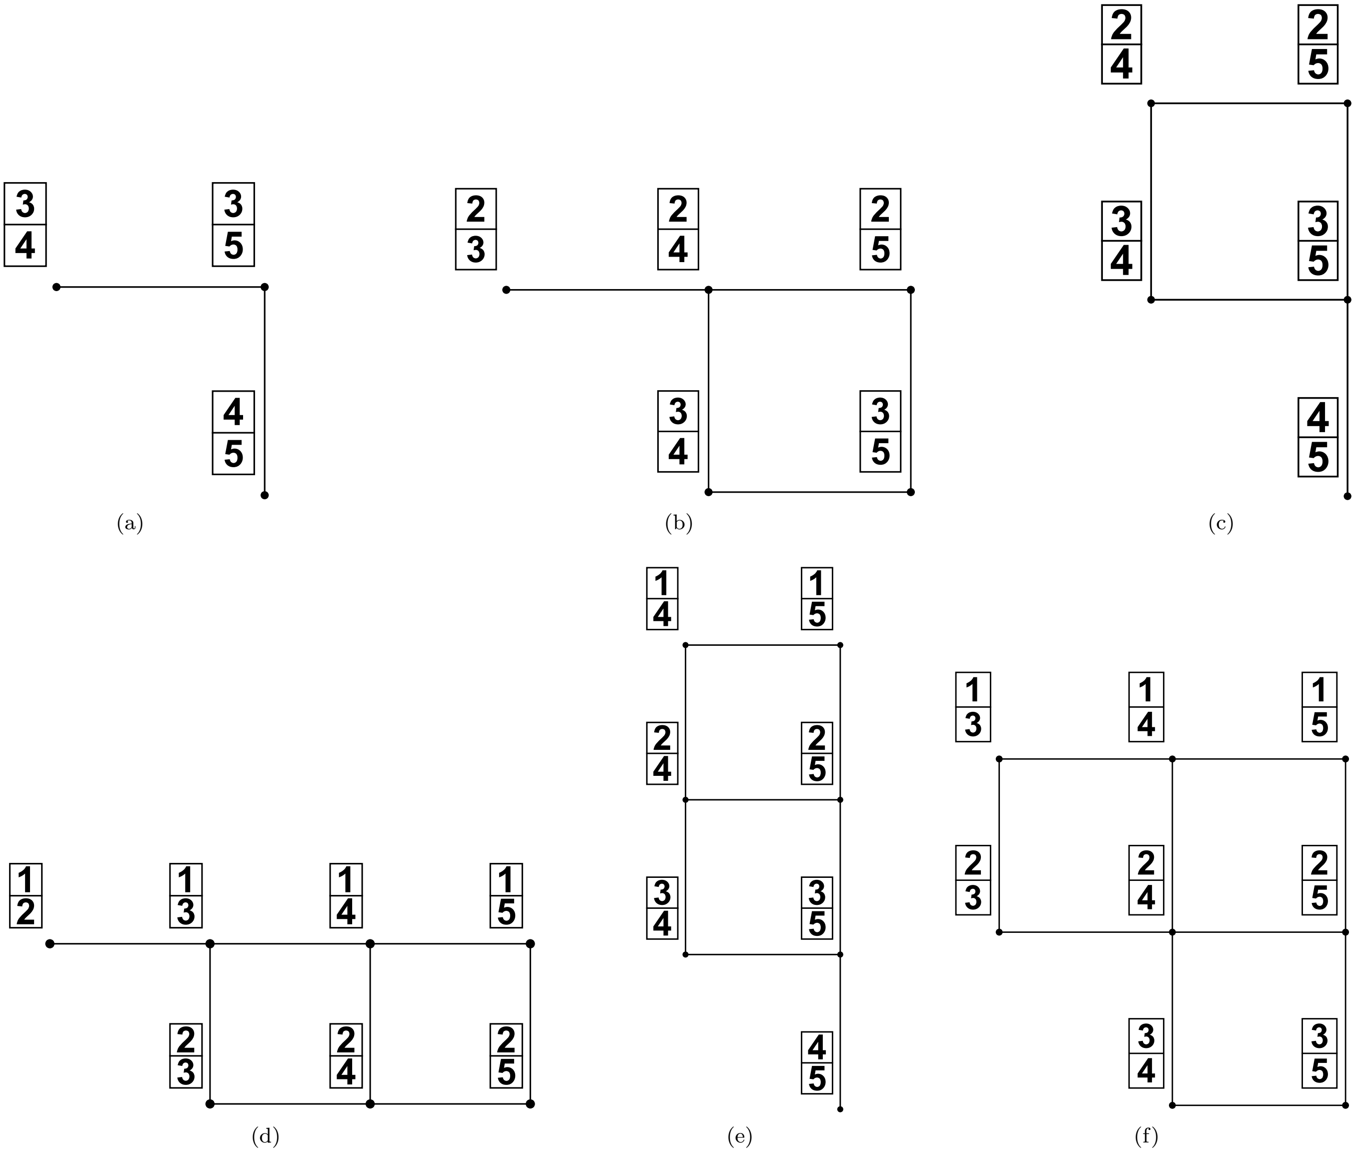


Figure S-3. Subgraphs associated to Eqs.(S-7)–(S-9).

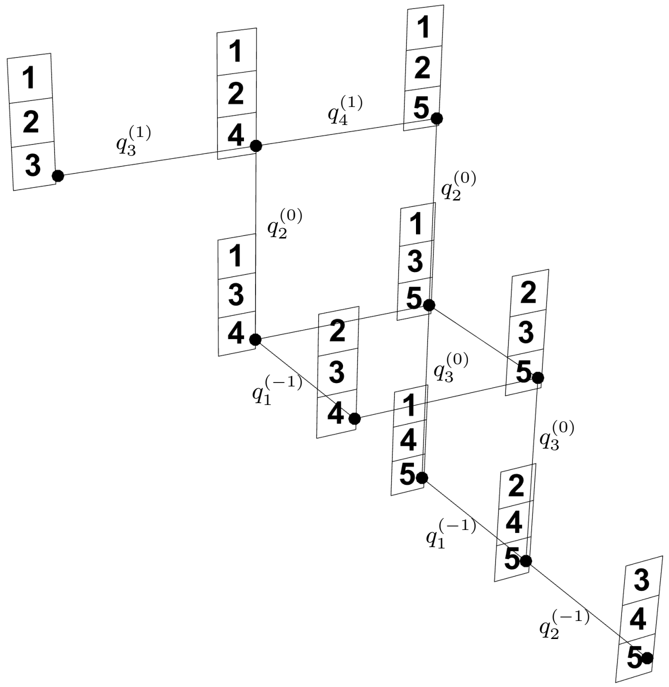


Figure S-4. Pole canceling graph of $sl_5$ for $a = 3$. In order to make the visualization clearer we did not write the $q$-functions corresponding to the poles by every edge. The edges without labels have the same set of poles $q_1^{(-1)}$ and $q_3^{(0)}$ as the parallel edges.

Finally, for the third representation we build the graph in Fig.S-4. The adjacency matrix is given by

$$A_{3,1}^{(5)}(x) = \begin{bmatrix} 0 & q_3^{(1)} & 0 & 0 & 0 & 0 & 0 & 0 & 0 & 0 \\ q_3^{(1)} & 0 & q_4^{(1)} & q_2^{(0)} & 0 & 0 & 0 & 0 & 0 & 0 \\ 0 & q_4^{(1)} & 0 & 0 & q_2^{(0)} & 0 & 0 & 0 & 0 & 0 \\ 0 & q_2^{(0)} & 0 & 0 & q_4^{(1)} & 0 & q_1^{(-1)} & 0 & 0 & 0 \\ 0 & 0 & q_2^{(0)} & q_4^{(1)} & 0 & q_3^{(0)} & 0 & q_1^{(-1)} & 0 & 0 \\ 0 & 0 & 0 & 0 & q_3^{(0)} & 0 & 0 & 0 & q_1^{(-1)} & 0 \\ 0 & 0 & 0 & q_1^{(-1)} & 0 & 0 & 0 & q_4^{(1)} & 0 & 0 \\ 0 & 0 & 0 & 0 & q_1^{(-1)} & 0 & q_4^{(1)} & 0 & q_3^{(0)} & 0 \\ 0 & 0 & 0 & 0 & 0 & q_1^{(-1)} & 0 & q_3^{(0)} & 0 & q_2^{(-1)} \\ 0 & 0 & 0 & 0 & 0 & 0 & 0 & 0 & q_2^{(-1)} & 0 \end{bmatrix}, \tag{S-10}$$

and polynomials

$$\begin{array}{|c|}\hline 1,2 \\ \hline 2,3 \\ \hline 3,4 \\ \hline \end{array}_{\,x} = \frac{\Phi_+(x+\mathrm{i})\Phi_-(x+\mathrm{i})\Phi_+(x)\Phi_-(x)\Phi_+(x-\mathrm{i})p_{3,1}^{(5)}(x)}{q_4(x+\mathrm{i})}, \quad \begin{array}{|c|}\hline 2,3 \\ \hline 3,4 \\ \hline 4,5 \\ \hline \end{array}_{\,x} = \frac{\Phi_-(x+\mathrm{i})\Phi_+(x)\Phi_-(x)\Phi_+(x-\mathrm{i})\Phi_-(x-\mathrm{i})p_{3,2}^{(5)}(x)}{q_1(x-\mathrm{i})}, \tag{S-11}$$

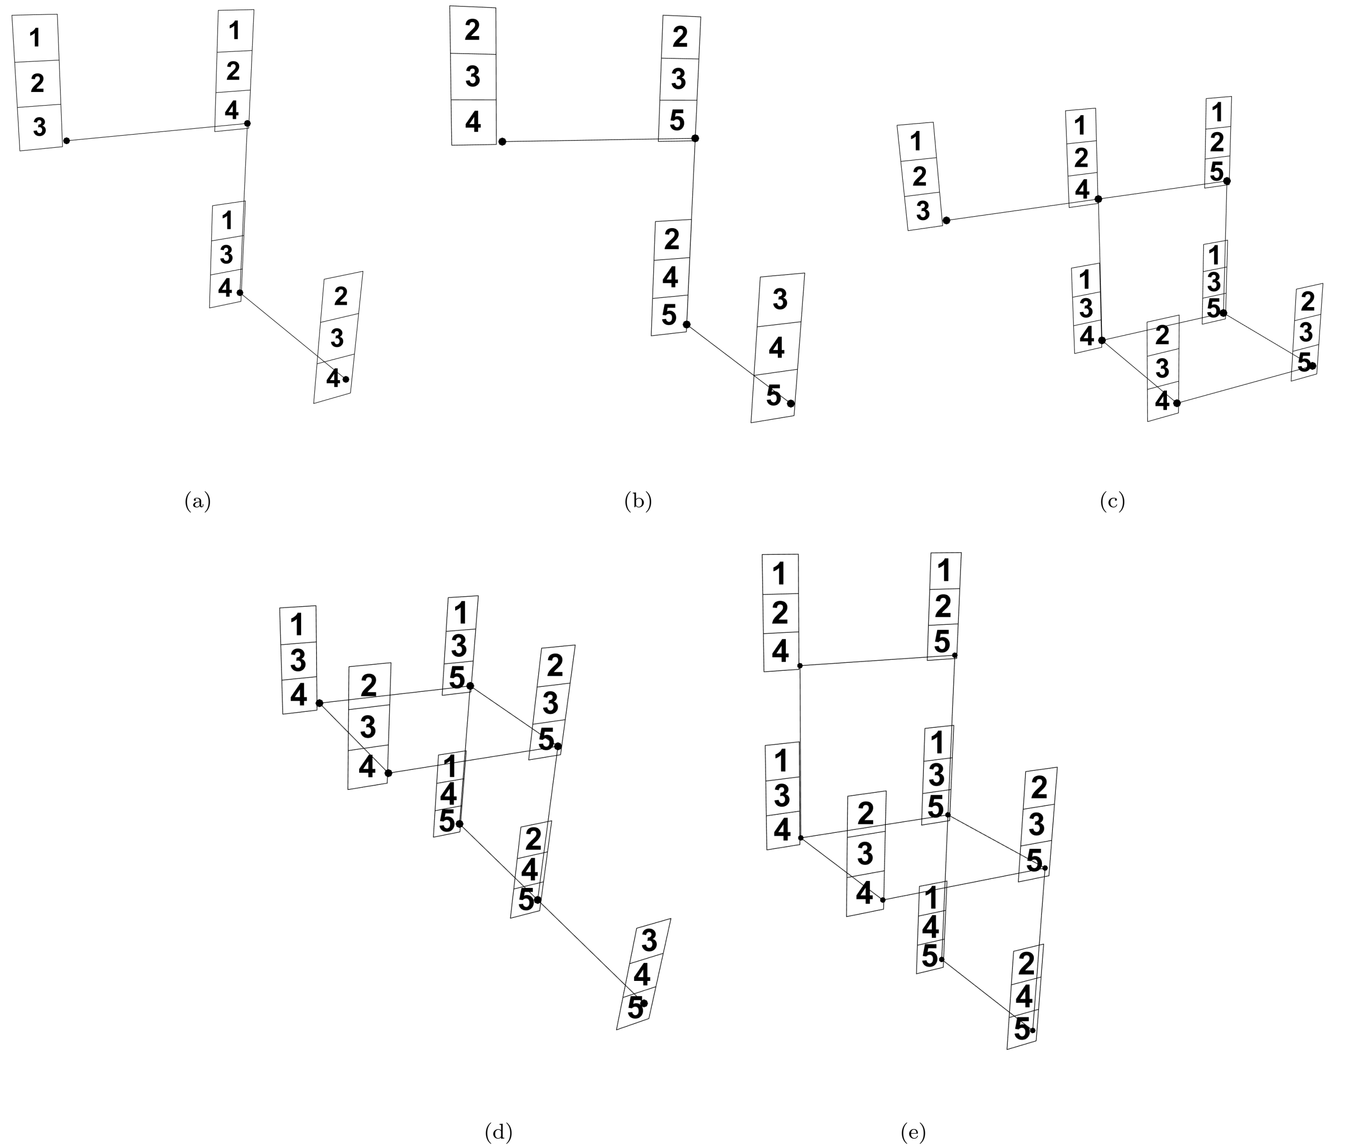


Figure S-5. Subgraphs associated to Eqs.(S-11)–(S-13).

$$\boxed{\begin{array}{c}1,2\\ \hline 2,3\\ \hline 3,5\end{array}}_{\,x} = \frac{\Phi_+(x-\mathrm{i})\Phi_-(x+\mathrm{i})\Phi_+(x)\Phi_-(x)p^{(5)}_{3,3}(x)}{q_3(x)}, \qquad \boxed{\begin{array}{c}1,3\\ \hline 3,4\\ \hline 4,5\end{array}}_{\,x} = \frac{\Phi_+(x-\mathrm{i})\Phi_-(x+\mathrm{i})\Phi_+(x)\Phi_-(x)p^{(5)}_{3,4}(x)}{q_2(x)}, \tag{S-12}$$

$$\boxed{\begin{array}{c}1,2\\ \hline 2,4\\ \hline 4,5\end{array}}_{\,x} = \frac{\Phi_+(x-\mathrm{i})\Phi_-(x+\mathrm{i})\Phi_+(x)\Phi_-(x)p^{(5)}_{3,5}(x)}{q_2(x-\mathrm{i})q_3(x+\mathrm{i})}. \tag{S-13}$$

Note that a graphical representation for the last representation would be four-dimensional. Therefore we simply

present the matrix, given by

$$A_{4,1}^{(5)}(x) = \begin{bmatrix} 0 & q_4^{(3/2)} & 0 & 0 & 0 \\ q_4^{(3/2)} & 0 & q_3^{(1/2)} & 0 & 0 \\ 0 & q_3^{(1/2)} & 0 & q_2^{(-1/2)} & 0 \\ 0 & 0 & q_2^{(-1/2)} & 0 & q_1^{(-3/2)} \\ 0 & 0 & 0 & q_1^{(-3/2)} & 0 \end{bmatrix}. \tag{S-14}$$

It is worth noting that all $sl_5$ graphs can be projected onto the plane since each vertex is connected at most to three other vertices. This feature facilitates the extraction of the EAFs from them. With the eigenvalues

$$\Lambda_{1,1}^{(5)}(x) = \begin{array}{|c|}\hline 1,5 \\ \hline \end{array}, \qquad \Lambda_{4,1}^{(5)}(x) = \begin{array}{|c|}\hline 1,2 \\ \hline 2,3 \\ \hline 3,4 \\ \hline 4,5 \\ \hline \end{array}, \tag{S-15}$$

plus the Bethe root functions $q_j(x),\ j = 1, \ldots, 4$, we have a complete set with 30 EAFs to be eliminated in order to find a nontrivial relation between the lowercase and uppercase auxiliary functions of $sl_5$.

The positions of the zeroes of the new polynomials on the complex plane are given in the table below.

| $p(x)$ | $\mathrm{Im}(x)$ |
|---|---|
| $q_4(x)$ | $0$ |
| $p_{1,j}^{(5)}(x),\ j = 6, \ldots, 9$ | $\pm 1$ |
| $p_{2,5}^{(5)}(x)$ | $\pm 3/2$ |
| $p_{2,j}^{(5)}(x),\ j = 6, 7$ | $+1/2,\ \pm 3/2$ |
| $p_{2,j}^{(5)}(x),\ j = 8, 9$ | $-1/2,\ \pm 3/2$ |
| $p_{2,10}^{(5)}(x)$ | $\pm 1/2,\ \pm 3/2$ |
| $p_{3,j}^{(5)}(x),\ j = 1, 2$ | $\pm 2$ |
| $p_{3,j}^{(5)}(x),\ j = 3, 4$ | $0, \pm 2$ |
| $p_{3,5}^{(5)}(x)$ | $\pm 1,\ \pm 2$ |
| $\underline{\Lambda}_{1,1}^{(5)}(x)$ | $\pm 1$ |
| $\underline{\Lambda}_{4,1}^{(5)}(x)$ | $\pm 5/2$ |

Table I. Positions of zeroes of the EAFs in the complex plane. These EAFs first appeared in the $sl(5)$ case.
